# Supplementary material for: Classification of Collective Modes in a Charge Density Wave by Momentum-Dependent Modulation of the Electronic Band Structure
Source: arXiv:1505.07350 source file (2015-05-27)
Supplement: Supplementary file 1 [file SOM.pdf]

# Supplemental Materials: Classification of Collective Modes in a Charge Density Wave by Momentum-Dependent Modulation of the Electronic Band Structure

D. Leuenberger,[1,2] J. A. Sobota,[1,2,3] S.-L. Yang,[1,2,4] A. F. Kemper,[3] P. Giraldo-Gallo,[1,2]
R. G. Moore,[1,2] I. R. Fisher,[1,2] P. S. Kirchmann,[1,*] T. P. Devereaux,[1,2] and Z.-X. Shen[1,2,4,†]
[1]*Stanford Institute for Materials and Energy Sciences,*
*SLAC National Accelerator Laboratory, 2575 Sand Hill Road, Menlo Park, CA 94025, USA*
[2]*Geballe Laboratory for Advanced Materials, Department of Applied Physics, Stanford University, Stanford, CA 94305, USA*
[3]*Lawrence Berkeley National Lab, 1 Cyclotron Road, Berkeley, CA 94720, USA*
[4]*Department of Physics, Stanford University, Stanford, CA 94305, USA*
(Dated: February 27, 2015)

## DETERMINATION OF FLUENCE AND DEPOSITED PUMP ENERGY PER UNIT CELL

This section describes how the absorbed optical excitation density per unit cell is quantified. The penetration depth $d_{h\nu}$ of an optical pump pulse with photon energy $h\nu$ and wavelength $\lambda$ amounts to

$$d_{h\nu} = \frac{\lambda}{4\pi \cdot \kappa(\lambda)} \quad , \tag{S1}$$

with $\kappa(\lambda)$ being the imaginary part of the complex refractive index $N$

$$N = n + i\kappa \quad . \tag{S2}$$

The complex dielectric function $\epsilon$ is written as

$$\epsilon = \epsilon' + i\epsilon'' = \epsilon' + i\frac{\sigma\lambda}{2\pi c} \quad , \tag{S3}$$

with the optical conductivity $\sigma(\lambda)$ in the imaginary part $\epsilon''$. The dielectric function $\epsilon$ is related to $N$ by

$$N^2\epsilon_0 = \epsilon \quad . \tag{S4}$$

Therefore, $\kappa$ can be written as

$$\kappa = \frac{\sigma\lambda}{4\pi\epsilon_0 c n} \quad . \tag{S5}$$

The real part $n$ and imaginary part $\kappa$ of the complex refractive index are related to the reflectivity $R(\lambda)$ through:

$$R = \left|\frac{1-N}{1+N}\right|^2 = \left[\frac{(1-n)^2+\kappa^2}{(1+n)^2+\kappa^2}\right] \quad . \tag{S6}$$

Combining Eq. (S5) and (S6) allows to compute $\kappa(\lambda)$ as function of the measured quantities $R(\lambda)$ and $\sigma(\lambda)$ obtained from optical reflectivity measurements [1]

$$\kappa^4 + \kappa^2 + \frac{(R+1)}{(R-1)}\frac{\sigma\lambda}{2\pi\epsilon_0 c}\kappa + \frac{\sigma^2\lambda^2}{16\pi 2\epsilon_0^2 c^2} = 0 \quad . \tag{S7}$$

Fig. S1 plots the polynomial in Eq. (S7) as function of $\kappa$ for different wavelengths $\lambda$ for $CeTe_3$ at 100 K. Within the measured wavelength range, Eq. (S7) reveals two solutions for $\kappa(\lambda)$. The *colored dots* mark the physical meaningful solution because continuous extension of those values matches with the single positive solution of Eq. (S7) for wavelengths below 820 nm.

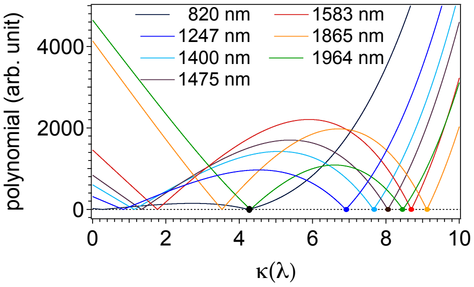


FIG. S1. Colored dots correspond to the calculated imaginary part of the refractive index $\kappa(\lambda)$ for $CeTe_3$ at 100 K.

The absorbed energy per unit cell $\epsilon_{uc}(z)$ decays exponentially as function of penetration depth $z$ normal to the sample surface

$$\epsilon_{uc}(z) = \epsilon_{1st} \cdot \exp\left(-z/d_{h\nu}\right) \quad . \tag{S8}$$

$\epsilon_{1st}$ denotes the absorbed energy within the 1st unit cell at $z = 0$ and is given by

$$\epsilon_{1st} = (1 - R(\lambda)) \cdot \ E_{h\nu} \cdot \frac{V_{uc}}{A' \cdot d_{h\nu}} \quad . \tag{S9}$$

$E_{h\nu}$ denotes the pump-pulse energy and $V_{uc} = 498.6$ Å$^3$ [2] is the size of the unit cell of $CeTe_3$. For 2D Gaussian beam profiles $a(x, y)$

$$a(x,y) \ = \ exp\left(-\left(\frac{(x-x_0)^2}{2\sigma_x^2} + \frac{(y-y_0)^2}{2\sigma_y^2}\right)\right) \tag{S10}$$

the area of the incident pulses on the sample $A'$ then amounts to

$$A' \ = \ \frac{\pi}{4\ln(2)} \cdot \frac{FWHM_x}{\cos(50^\circ - \theta)} \cdot \frac{FWHM_y}{\cos(\phi)} \quad . \tag{S11}$$

$\theta$ ($\phi$) corresponds to the angle between sample surface normal and horizontal (vertical) direction of detection. $FWHM_x$ ($FWHM_y$) is the horizontal (vertical)

full-width half-maximum of the beam profile at normal incidence. Here, the photon energy of the pump-pulses (1.0 eV) is smaller than the electronic band gap of common Si-CCD detectors (~1.1 eV). Therefore, we determine the beam profiles by a knife-edge measurement. Accuracy of this method is cross-checked by comparison to measurements with a Si-CCD detector, at a wavelength of 820 nm ($h\nu = 1.5$ eV), which can be detected by both techniques.

Finally, in order to obtain absorbed energy per unit cell averaged over the probed sample region $\epsilon$, we integrate $\epsilon_{h\nu}(z)$ weighted by the electron mean free path $d_{6eV}$ of our 6 eV probe pulse:

$$\epsilon = \frac{\int_0^\infty \epsilon_{1st} \exp\left(-z/d_{h\nu}\right) \exp\left(-z/d_{6eV}\right) dz}{\int_0^\infty \exp\left(-z/d_{6eV}\right) dz} \quad \text{(S12)}$$

$$= \frac{\epsilon_{1st}}{1 + \left(\frac{d_{6eV}}{d_{h\nu}}\right)} . \quad \text{(S13)}$$

Together with $d_{6eV} = 4 \pm 2\ nm$, $d_{h\nu} = d_{1eV} = 14.4 \pm 0.2\ nm$ and $k(\lambda = 1245\ nm) = 6.9$, we obtain with Eq. (S13) the fluence values listed in Table S1.

| ($\mu$J cm$^{-2}$) | (meV) |
|---|---|
| 55 ± 6 | 16 ± 2 |
| 95 ± 11 | 28 ± 3 |
| 152 ± 17 | 44 ± 5 |
| 245 ± 28 | 72 ± 8 |
| 354 ± 40 | 103 ± 12 |

TABLE S1. Experimental values of the absorbed pump-pulse fluence ($\mu$Jcm$^{-2}$) and the absorbed energy per $CeTe_3$ unit cell (meV), at 1.0 eV photon energy.

By considering the errors $m_{d_{h\nu}}$, $m_{d_{6eV}}$ and $m_{\epsilon_{1st}}$ we obtain the error bars $m_\epsilon$ for the absorbed energy $\epsilon$ listed in Table S1 with

$$m_\epsilon^2 = \left(\frac{\epsilon}{\epsilon_{1st}} m_{\epsilon_{1st}}\right)^2 + \left(\frac{-\epsilon}{d_{h\nu} + d_{6eV}} m_{d_{6eV}}\right)^2 + \left(\epsilon \left(\frac{d_{h\nu}^2}{d_{6eV}} + d_{h\nu}\right)^{-1} m_{d_{h\nu}}\right)^2 . \quad \text{(S14)}$$

The error of $\epsilon_{1st}$ depends on the error of the measured spot size $A'$ and pump-pulse energy $E_{h\nu}$ as following

$$\left(\frac{m_{\epsilon_{1st}}}{\epsilon_{1st}}\right)^2 = \sum_{i=x,y} \left(\frac{m_{FWHM_i}}{FWHM_i}\right)^2 + \left(\frac{m_{E_{h\nu}}}{E_{h\nu}}\right)^2 . \quad \text{(S15)}$$

## FLUENCE DEPENDENCE OF THE CDW GAP

The maximum reduction of $2\Delta$ normalised by the equilibrium value of $2\Delta$ at negative pump-probe delays leads to the $\delta\Delta/\Delta$, plotted as function of fluence and absorbed energy per unit cell in Fig. S2. Within this perturbative excitation regime, the maximum decrease of $2\Delta$ depends linearly on the excitation density.

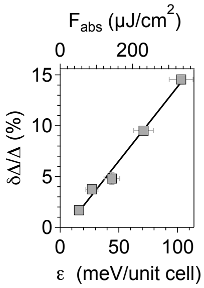


FIG. S2. $\delta\Delta/\Delta$ at 100 K is plotted as function of absorbed fluence $F_{abs}$ or absorbed energy $\epsilon$ per unit cell (*markers*) and fitted by a linear function (*line*).

## FREQUENCY DETERMINATION

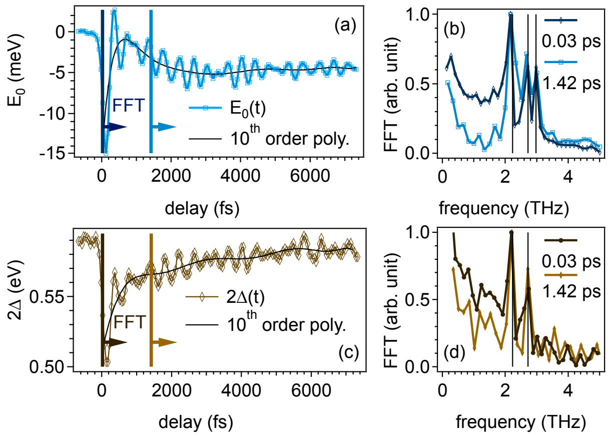


FIG. S3. (a) Rigid energy shift $E_0(t)$ and (c) CDW gap size $2\Delta(t)$ as function of pump-probe delay. *Vertical bars* indicate different starting points for the corresponding FT in (b) and (d). *Solid line* is a $10^{th}$ order polynomial fitted to the data.

Variation of the starting point for the Fourier Transform (FT) of $E_0(t)$ and $2\Delta(t)$ between 0 ps and 1.4 ps, marked as vertical bars in Fig. S3 (a), does not change the frequencies of the three main modes $\Omega_1$, $\Omega_2$ and $\Omega_3$ in Fig. S3 (b). We subtract a $10^{th}$ order polynomial fit from $E_0(t)$ to extract the oscillatory modifications even more clearly. This procedure is legitimate since the number of possible nodes of the $10^{th}$ order polynomial is much smaller than the number of oscillation periods analyzed. Furthermore, the FT of $\delta E_0(t)$ in Fig. S4 reveals the same dominant frequencies $\Omega_1$, $\Omega_2$ and $\Omega_3$ as for $E_0(t)$ in Fig. S3 (b). The same argument for background subtraction applies for $2\Delta(t)$ and the two modes $\Omega_1$ and $\Omega_2$, displayed in Fig. S3 (c) and (d).

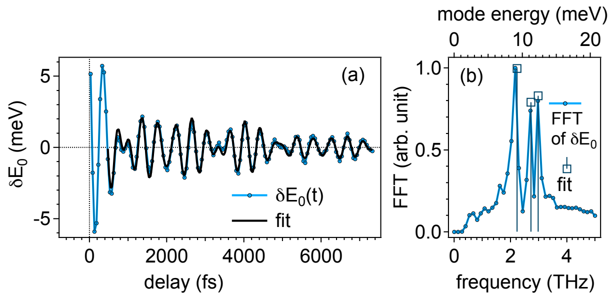


FIG. S4. Subtraction of the fitted background from $E_0(t)$ leads to $\delta E_0(t)$ in (a) (*markers*). *Solid line* in (a) denotes the fit of Eq. (S16) to $\delta E_0(t)$. The resulting frequencies $\Omega_i$ (*vertical bars*) and amplitudes $A_i$ (*markers*) match the corresponding FT of $\delta E_0(t)$ in (b).

Additionally, the frequencies of the dominant modes $\Omega_1$=2.23(1) THz, $\Omega_2$=2.72(1) THz and $\Omega_3$=2.98(1) THz have been obtained from fitting the following form

$$\delta E_0(t) = \sum_{i=1}^{3} A_i e^{(-t/\tau_i)} cos(2\pi\Omega_i t + \phi_i) \qquad \text{(S16)}$$

to the residual rigid energy shift $\delta E_0(t)$. Fitting many oscillation periods with cosine functions is highly constraining on the frequencies $\Omega_i$. $A_i$ denotes the oscillatory strength, $\phi_i$ the phase and $\tau_i$ the damping time of each mode with frequency $\Omega_i$.

$\Omega_i$ and $A_i$ from the fit in Fig. S4 (a) are marked as *vertical lines* and *markers* in Fig. S4 (b) and match the three prominent features in the corresponding FT. The fitted values for $\Omega_i$, $\phi_i$ and $\tau_i$ are listed in Table S2. The phases $\phi_2$ and $\phi_3$ are close to zero, which is conventionally attributed to the displacive excitation of optical phonons [3].

| $\Omega_i$ | frequency (THz) | $\phi_i$ (degree) | $\tau_i$ (ps) |
|---|---|---|---|
| $\Omega_1$ | 2.23 ± 0.01 | 14 ± 2 | 4.9 ± 0.3 |
| $\Omega_2$ | 2.72 ± 0.01 | -4 ± 5 | 3.6 ± 0.4 |
| $\Omega_3$ | 2.98 ± 0.01 | 5 ± 5 | 4.0 ± 0.5 |

TABLE S2. Frequencies $\Omega_i$, phases $\phi_i$ and damping constants $\tau_i$ of the three dominant modes.

## K-DEPENDENT OSCILLATORY RESPONSE

Fig. 4 in the main text presents the momentum-resolved response of the three modes $\Omega_1$, $\Omega_2$ and $\Omega_3$. This paragraph explains the model-free analysis in detail. Fig. S5 (a) presents an energy versus momentum cut at a fixed delay of -330 fs. First, we analyze the oscillatory response of the Te-5$p$ binding energy at a fixed point in $k$-space by looking at a single spectrum, indicated by a vertical *red line* in Fig. S5 (a). We fit the band position at this particular $\vec{k}$ with a Gaussian function (*dashed line* in (b)) and extract the corresponding change in binding energy $\delta E_{bin}(t, \vec{k} = const)$ for each delay, as shown in Fig. S5 (c). We then perform this analysis for all $\vec{k}$. FT of $\delta E_{bin}(t, \vec{k} = const)$ for all measured momenta $\vec{k}$ leads to the false-color plot in Fig. S5 (d) for the highest pump fluence of 103 meV per unit cell. The horizontal *dashed lines* highlight the response of the dominant modes $\Omega_1$, $\Omega_2$ and $\Omega_3$. This procedure leads to the panels in Fig. 4 of the main manuscript. In order to crosscheck the transient fit of the TB dispersion to the data, the same model-free analysis was applied to the fitted TB band structure for all delays and pump fluences. The resulting momentum dependent oscillation strengths are plotted in Fig. 4 of the main text.

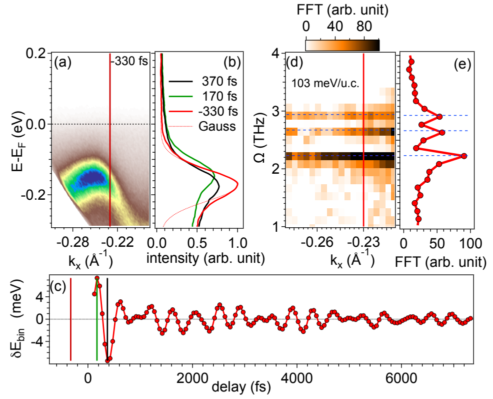


FIG. S5. (a) Energy versus momentum cut at -330 fs delay displays the occupied Te-5$p$ band. *Vertical red line* indicates the momentum position of the spectra in (b). Spectra in (b) for different delays at fixed $\vec{k}$ are fitted by a Gaussian (*dotted line*) and lead to the change in binding energy $\delta E_{bin}(t, \vec{k} = const)$ in (c). FT of $\delta E_{bin}(t)$ as function of momentum leads to the frequency versus momentum plot in (d). *Dashed lines* highlight the dominant modes $\Omega_1$, $\Omega_2$ and $\Omega_3$. The *vertical line* indicates the FT plotted in (e).

## DFT NORMAL STATE BAND STRUCTURE

Fig. S6 displays DFT band calculations of the normal state in $CeTe_3$. With increasing atomic displacement of $\mu/b = 0.5$ % along the out-of-plane $A_{1g}$ mode the Te-5$p_{x,z}$ band shifts linearly in energy.

* kirchman@stanford.edu
† zxshen@stanford.edu

[1] B. F. Hu, P. Zheng, R. H. Yuan, T. Dong, B. Cheng, Z. G. Chen, and N. L. Wang, Phys. Rev. B **83**, 155113 (2011).
[2] N. Ru, C. L. Condron, G. Y. Margulis,

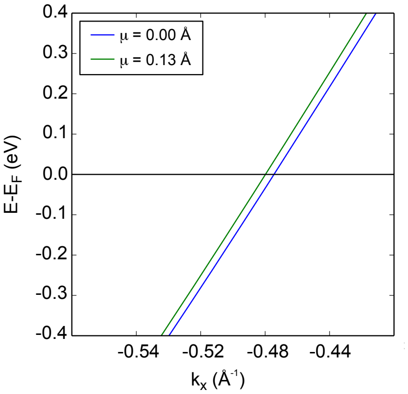


FIG. S6. DFT calculation of the normal state band dispersion in $CeTe_3$. Bands are plotted along the Γ-X direction with $k_z$= 0 $Å^{-1}$, for the undistorted case (*blue line*) and for an atomic displacement of $\mu = 0.13$ Å in the out-of-plane $A_{1g}$ mode (*green line*).

K. Y. Shin, J. Laverock, S. B. Dugdale, M. F. Toney, and I. R. Fisher, Phys. Rev. B **77**, 035114 (2008).
[3] H. J. Zeiger, J. Vidal, T. K. Cheng, E. P. Ippen, G. Dresselhaus, and M. S. Dresselhaus, Phys. Rev. B **45**, 768 (1992).
